# Supplementary material for: Contrastive Positive Sample Propagation along the Audio-Visual Event Line
Source: arXiv:2211.09980 source file (2022-11-18)
Supplement: Supplementary file 1 [file appendix.tex]

\section*{Appendex}

\section{Implementation Details of ISDA. }
\label{grad}
\textbf{Dynamic estimation of covariance matrices.}
During the training process using $\overline{\mathcal{L}}_{\infty}$, covariance matrices are estimated by:
\begin{equation}
    \label{ave}
    \bm{\mu}_j^{(t)} = \frac{n_j^{(t-1)}\bm{\mu}_j^{(t-1)} + m_j^{(t)} {\bm{\mu}'}_j^{(t)}}
    {n_j^{(t-1)} +m_j^{(t)}},
\end{equation}
\begin{equation}
    \label{cv}
    \begin{split}
        \Sigma_j^{(t)} 
         = \frac{n_j^{(t-1)}\Sigma_j^{(t-1)} + m_j^{(t)} {\Sigma'}_j^{(t)}}
        {n_j^{(t-1)} +m_j^{(t)}} 
         + \frac{n_j^{(t-1)}m_j^{(t)} (\bm{\mu}_j^{(t-1)} - {\bm{\mu}'}_j^{(t)})
        (\bm{\mu}_j^{(t-1)} - {\bm{\mu}'}_j^{(t)})^T}
        {(n_j^{(t-1)} +m_j^{(t)})^2},
    \end{split}
\end{equation}
\begin{equation}
    \label{sum}
    n_j^{(t)} = n_j^{(t-1)} + m_j^{(t)}
\end{equation}
where $\bm{\mu}_j^{(t)}$ and $\Sigma_j^{(t)}$ are the estimates of average values and covariance matrices of the features of $j^{th}$ class at $t^{th}$ step. ${\bm{\mu}'}_j^{(t)}$ and ${\Sigma'}_j^{(t)}$ are the average values and covariance matrices of the features of $j^{th}$ class in $t^{th}$ mini-batch. $n_j^{(t)}$ denotes the total number of training samples belonging to $j^{th}$ class in all $t$ mini-batches,
and $m_j^{(t)}$ denotes the number of training samples belonging to $j^{th}$ class only in $t^{th}$ mini-batch. 

% In addition, as the covariance is estimated according to the network's current outputs, it makes little sense to apply ISDA loss in the beginning of the training process, when models have not learned linearized deep representations. Therefore, we adopts a smooth transit from the standard cross-entropy to ISDA loss by linearly increasing the weight of the estimated covariance matrices:
% \begin{equation}
%     \label{dynamicCV}
%     \Sigma_{i} = \lambda \frac{t}{T} \bm{M}_{y_{i}}^{(t)},
% \end{equation}
% where $T$ is the total number of training steps, and $\lambda$ is a hyper-parameter to adjust the scale of covariance matrices.

\textbf{Gradient computation.} In backward propagation, gradients of $\overline{\mathcal{L}}_{\infty}$ are given by:
\begin{equation}
    \label{g_1}
    \frac{\partial{\overline{\mathcal{L}}_{\infty}}}{\partial b_j} =
    \frac{\partial{\overline{\mathcal{L}}_{\infty}}}{\partial z_j} = 
    \begin{cases}
        \frac{e^{z_{y_i}}}{\sum_{j=1}^{C}e^{z_{j}}}-1, &j = y_i \\
        \frac{e^{z_{j}}}{\sum_{j=1}^{C}e^{z_{j}}}, &j \neq y_i 
    \end{cases},
\end{equation}
\begin{equation}
    \label{g_2}
    \frac{\partial{\overline{\mathcal{L}}_{\infty}}}{\partial \bm{w}^{T}_{j}} = 
    \begin{cases}
        (\bm{a}_{i} + \sum_{n=1}^{C}[(\bm{w}^{T}_{n} - \bm{w}^{T}_{y_{i}})\Sigma_{i}])
        \frac{\partial{\overline{\mathcal{L}}_{\infty}}}{\partial z_j}, &j = y_i \\
        (\bm{a}_{i} + (\bm{w}^{T}_{j} - \bm{w}^{T}_{y_{i}})\Sigma_{i})
        \frac{\partial{\overline{\mathcal{L}}_{\infty}}}{\partial z_j},  &j \neq y_i 
    \end{cases},
\end{equation}
\begin{equation}
    \label{g_3}
    \frac{\partial{\overline{\mathcal{L}}_{\infty}}}{\partial a_k} = \sum_{j=1}^{C} 
    w_{jk} \frac{\partial{\overline{\mathcal{L}}_{\infty}}}{\partial z_j}, 1 \leq k \leq A,
\end{equation}
where $w_{jk}$ denotes $k^{th}$ element of $\bm{w}_{j}$. ${\partial{\overline{\mathcal{L}}_{\infty}}}/{\partial \bm{\Theta}}$ can be obtained through the backward propagation algorithm using ${\partial{\overline{\mathcal{L}}_{\infty}}}/{\partial \bm{a}}$.

\section{Training Details}
On CIFAR, we implement the ResNet, SE-ResNet, Wide-ResNet, ResNeXt, DenseNet and PyramidNet.
The SGD optimization algorithm with a Nesterov momentum is applied to train all models. Specific hyper-parameters for training are presented in Table \ref{Training_hp}.

\begin{table*}[h]
	\scriptsize
    \centering
    \vskip -0.2in
    \caption{Training configurations on CIFAR. `$l_r$' donates the learning rate.}
    \label{Training_hp}
    \setlength{\tabcolsep}{0.5mm}{
    \vspace{5pt}
     
    \begin{tabular}{c|c|c|c|c|c|c}
    \hline
    Network & Total Epochs & Batch Size & Weight Decay & Momentum & Initial $l_r$ & $l_r$ Schedule \\
    \hline
    ResNet & 160 & 128 & 1e-4 & 0.9 & 0.1 & Multiplied by 0.1 in $80^{th}$ and $120^{th}$ epoch. \\
    \hline
    SE-ResNet & 200 & 128 & 1e-4 & 0.9 & 0.1 & Multiplied by 0.1 in $80^{th}$, $120^{th}$ and $160^{th}$ epoch. \\
    \hline
    Wide-ResNet & 240 & 128 & 5e-4 & 0.9 & 0.1 & Multiplied by 0.2 in $60^{th}$, $120^{th}$, $160^{th}$ and $200^{th}$ epoch. \\
    \hline
    DenseNet-BC & 300 & 64 & 1e-4 & 0.9 & 0.1 & Multiplied by 0.1 in $150^{th}$, $200^{th}$ and $250^{th}$ epoch. \\
    \hline
    ResNeXt & 350 & 128 & 5e-4 & 0.9 & 0.05 & Multiplied by 0.1 in $150^{th}$, $225^{th}$ and $300^{th}$ epoch. \\
    \hline
    Shake Shake &\multirow{1}{*}{1800}&\multirow{1}{*}{64}&\multirow{1}{*}{1e-4}&\multirow{1}{*}{0.9}&\multirow{1}{*}{0.1}&\multirow{1}{*}{Cosine learning rate.} \\
    % (CIFAR-10)& & & & & & \\
    % \hline
    % Shake Shake &\multirow{1}{*}{1800}&\multirow{2}{*}{128}&\multirow{2}{*}{1e-4}&\multirow{2}{*}{0.9}&\multirow{2}{*}{0.2}&\multirow{2}{*}{Cosine learning rate.} \\
    % (CIFAR-100)& & & & & & \\
    \hline
    PyramidNet &\multirow{1}{*}{1800}&\multirow{1}{*}{128}&\multirow{1}{*}{1e-4}&\multirow{1}{*}{0.9}&\multirow{1}{*}{0.1}&\multirow{1}{*}{Cosine learning rate.} \\
    % (CIFAR-100)& & & & & & \\

    % \multirow{2}{*}{Method} & \multicolumn{2}{c|}{ResNet-110} & \multicolumn{2}{c}{
        % Wide-ResNet-28-10}\\
    % &  CIFAR-10  &  CIFAR-100  &  CIFAR-10  &  CIFAR-100\\
    % \hline
    % Large Margin \cite{liu2016large} & 6.46$\pm$0.20\% & 28.00$\pm$0.09\% & 3.69$\pm$0.10\% & 18.48$\pm$0.05\%\\
    % Disturb Label \cite{Xie2016DisturbLabelRC} & 6.61$\pm$0.04\% & 28.46$\pm$0.32\% & 3.91$\pm$0.10\%& 18.56$\pm$0.22\%\\
    % Focal Loss \cite{Lin2017FocalLF} & 6.68$\pm$0.22\% & 28.28$\pm$0.32\% & 3.62$\pm$0.07\% & 18.22$\pm$0.08\%\\
    % Center Loss \cite{wen2016discriminative} & 6.38$\pm$0.20\% & 27.85$\pm$0.10\% & 3.76$\pm$0.05\% & {18.50$\pm$0.25\%}\\
    % L$_q$ Loss \cite{Zhang2018GeneralizedCE} & 6.69$\pm$0.07\% & 28.78$\pm$0.35\% & 3.78$\pm$0.08\% & 18.43$\pm$0.37\%\\
    % \hline
    % WGAN \cite{arjovsky2017wasserstein} & 6.63$\pm$0.23\% & - & 3.81$\pm$0.08\% & -\\
    % CGAN \cite{mirza2014conditional} & 6.56$\pm$0.14\% & 28.25$\pm$0.36\% & 3.81$\pm$0.11\% & $\pm$\%\\
    % ACGAN \cite{odena2017conditional} & 6.32$\pm$0.12\% & 28.48$\pm$0.44\% & 3.85$\pm$0.07\% & $\pm$\%\\
    % infoGAN \cite{chen2016infogan} & 6.59$\pm$0.12\% & 27.64$\pm$0.14\% & 3.93$\pm$0.04\% & $\pm$\%\\
    % \hline
    % Basic & 6.76$\pm$0.34\% & 28.67$\pm$0.44\% & - & -\\
    % Basic + Dropout & {6.23$\pm$0.11\%} & {27.11$\pm$0.06\%} & 3.82$\pm$0.15\% & 18.53$\pm$0.07\%\\
    % ISDA & 6.33$\pm$0.19\% & 27.57$\pm$0.46\% & - & -\\
    % ISDA + Dropout & \textbf{5.98$\pm$0.20\%} & \textbf{26.35$\pm$0.30\%} & \textbf{3.58$\pm$0.15\%} & \textbf{17.98$\pm$0.15\%}\\
    \hline
    \end{tabular}}
    % \vskip -0.3in
\end{table*}

% (1) ResNet \& SE-ResNet. Total epochs: 200; Batch size: 128; L2 weight decay: 1e-4; Initial learning rate: 0.1; The learning rate is multiplied by 0.1 in $80^{th}$, $120^{th}$ and $160^{th}$ epoch.

% (2)Wide-ResNet. Total epochs:240; Batch size: 128; L2 weight decay: 5e-4; Initial learning rate: 0.1; The learning rate is multiplied by 0.2 in $60^{th}$, $120^{th}$, $160^{th}$ and $200^{th}$ epoch.

% (3)DenseNet-BC. Total epochs:300; Batch size: 64; L2 weight decay: 1e-4; Initial learning rate: 0.1; The learning rate is multiplied by 0.1 in $150^{th}$, $200^{th}$ and $250^{th}$ epoch.

% (3)ResNeXt. Total epochs:350; Batch size: 128; L2 weight decay: 1e-4; Initial learning rate: 0.1; The learning rate is multiplied by 0.1 in $150^{th}$, $200^{th}$ and $250^{th}$ epoch.

% The models are trained using the SGD optimization algorithm with a l2 weight decay of 1e-4 and a momentum of 0.9. The initial learning rate is set as 0.1 and divided by 10 in $80^{th}$ and $120^{th}$ epoch of total 160 epochs for ResNet based models, and in $150^{th}$ and $200^{th}$ epoch of total 300 epoch for DenseNet. The size of mini-batch is set as 128 for ResNet based models and 64 for DenseNet.
% Wide-ResNet is adopted with dropout rate of 0.3, following \cite{Zagoruyko2016WideRN}, while no dropout module is applied in ResNet and SE-ResNet. DenseNet is adopted with a dropout rate of 0.2, following \cite{2016arXiv160806993H}.

On ImageNet, we train ResNet for 120 epochs using the same l2 weight decay and momentum as CIFAR, following \cite{huang2016deep}. The initial learning rate is set as 0.1 and divided by 10 every 30 epochs. The size of mini-batch is set as 256.

All baselines are implemented with the same training configurations mentioned above.
% , except for the center loss.
Dropout rate is set as 0.3 for comparison if it is not applied in the basic model, following the instruction in \cite{Srivastava2014DropoutAS}. For noise rate in disturb label, 0.05 is adopted in Wide-ResNet-28-10 on both CIFAR-10 and CIFAR-100 datasets and ResNet-110 on CIFAR 10, while 0.1 is used for ResNet-110 on CIFAR 100. Focal Loss contains two hyper-parameters $\alpha$ and $\gamma$. Numerous combinations have been tested on the validation set and we ultimately choose $\alpha=0.5$ and $\gamma=1$ for all four experiments. 
For L$_q$ loss, although \cite{Zhang2018GeneralizedCE} states that $q=0.7$ achieves the best performance in most conditions, we suggest that $q=0.4$ is more suitable in our experiments, and therefore adopted.
For center loss, we find its performance is largely affected by the learning rate of the center loss module, therefore its initial learning rate is set as 0.5 for the best generalization performance.

For generator-based augmentation methods, we apply the GANs structures introduced in \cite{arjovsky2017wasserstein, mirza2014conditional, odena2017conditional, chen2016infogan} to train the generators. 
For WGAN, a generator is trained for each class in CIFAR-10 dataset. For CGAN, ACGAN and infoGAN, a single model is simply required to generate images of all classes. A 100 dimension noise drawn from a standard normal distribution is adopted as input, generating images corresponding to their label. Specially, infoGAN takes additional input with two dimensions, which represent specific attributes of the whole training set. Synthetic images are involved with a fixed ratio in every mini-batch. Based on the experiments on the validation set, the proportion of generalized images is set as $1/6$.

\section{Reversing Convolutional Networks}

To explicitly demonstrate the semantic changes generated by ISDA, we propose an algorithm to map deep features back to the pixel space. Some extra visualization results are shown in Figure \ref{Extra}.
% The results are shown in Figure 

An overview of the algorithm is presented in Figure \ref{Reversing}.
As there is no closed-form inverse function for convolutional networks like ResNet or DenseNet, the mapping algorithm acts in a similar way to \cite{mahendran2015understanding} and \cite{Upchurch2017DeepFI}, by fixing the model and adjusting inputs to find images corresponding to the given features. However, given that ISDA augments semantics of images in essence, we find it insignificant to directly optimize the inputs in the pixel space. Therefore, we add a fixed pre-trained generator $\mathcal{G}$, which is obtained through training a wasserstein GAN \cite{arjovsky2017wasserstein}, to produce images for the classification model, and optimize the inputs of the generator instead. This approach makes it possible to effectively reconstruct images with augmented semantics.

\begin{figure*}
    % \vskip 0.2in
    \begin{center}
    \centerline{\includegraphics[width=\columnwidth]{Reverse_Algorithm.pdf}}
    \caption{Overview of the algorithm. We adopt a fixed generator $\mathcal{G}$ obtained by training a wasserstein gan to generate fake images for convolutional networks, and optimize the inputs of $\mathcal{G}$ in terms of the consistency in both the pixel space and the deep feature space.}
    \label{Reversing}
    \end{center}
    \vskip -0.2in
\end{figure*}

\begin{figure*}
    % \vskip 0.2in
    \begin{center}
    \centerline{\includegraphics[width=\columnwidth]{extra_result.pdf}}
    \caption{Extra visualization results.}
    \label{Extra}
    \end{center}
    \vskip -0.3in
\end{figure*}

The mapping algorithm can be divided into two steps:

\textbf{Step I. }Assume a random variable $\bm{z}$ is normalized to $\hat{\bm{z}}$ and input to $\mathcal{G}$, generating fake image $\mathcal{G}(\hat{\bm{z}})$. $\bm{x}_{i}$ is a real image sampled from the dataset (such as CIFAR). $\mathcal{G}(\hat{\bm{z}})$ and $\bm{x}_{i}$ are forwarded through a pre-trained convolutional network to obtain deep feature vectors $f(\mathcal{G}(\hat{\bm{z}}))$ and $\bm{a}_{i}$. The first step of the algorithm is to find the input noise variable $\bm{z}_{i}$ corresponding to $\bm{x}_{i}$, namely 
\begin{equation}
    \label{ra1}
    \bm{z}_{i} = \arg\min_{\bm{z}} \|f(\mathcal{G}(\hat{\bm{z}})) - \bm{a}_{i}\|_{2}^{2} +
    \eta\|\mathcal{G}(\hat{\bm{z}}) - \bm{x}_{i}\|_{2}^{2},\
    s.t.\ \hat{\bm{z}} = \frac{\bm{z} - \overline{\bm{z}}}{std(\bm{z})},
\end{equation}
where $ \overline{\bm{z}}$ and $std(\bm{z})$ are the average value and the standard deviation of $\bm{z}$, respectively.
The consistency of both the pixel space and the deep feature space are considered in the loss function, and we introduce a hyper-parameter $\eta$ to adjust the relative importance of two objectives.

\textbf{Step II. }We augment $\bm{a}_{i}$ with ISDA, forming $\tilde{\bm{a}}_{i}$ and reconstructe it in the pixel space. Specifically, we search for $\bm{z}_{i}'$ corresponding to $\tilde{\bm{a}}_{i}$ in the deep feature space, with the start point $\bm{z}_{i}$ found in Step I:
\begin{equation}
    \label{ra2}
    \bm{z}_{i}' = \arg\min_{\bm{z'}} \|f(\mathcal{G}(\hat{\bm{z}}')) - \tilde{\bm{a}}_{i}\|_{2}^{2},\
    s.t.\ \hat{\bm{z}}' = \frac{\bm{z'} - \overline{\bm{z'}}}{std(\bm{z'})}.
\end{equation}
As the mean square error in the deep feature space is optimized to 0, $\mathcal{G}(\hat{\bm{z}_{i}}')$
is supposed to represent the image corresponding to $\tilde{\bm{a}}_{i}$.

The proposed algorithm is performed on a single batch. In practice, a ResNet-32 network is used as the convolutional network. We solve Eq. (\ref{ra1}), (\ref{ra2}) with a standard gradient descent (GD) algorithm of 10000 iterations. The initial learning rate is set as 10 and 1 for Step I and Step II respectively, and is divided by 10 every 2500 iterations. We apply a momentum of 0.9 and a l2 weight decay of 1e-4.

\section{Extra Experimental Results}

\begin{figure}[htp]
    % \vskip 0.2in
    \begin{center}
    \subfigure[ResNet-110 on CIFAR-10]{
        \label{fig:evaluationC10}
    \includegraphics[width=0.45\columnwidth]{Re110C10.pdf}
    }
    \subfigure[ResNet-110 on CIFAR-100]{
        \label{fig:evluationC100}
    \includegraphics[width=0.45\columnwidth]{Re110C100.pdf}}
    % \subfigure[Wide-ResNet-28-10 on CIFAR-10+]{
    %     \label{fig:evluationC100}
    % \includegraphics[width=0.45\columnwidth]{wrnc10.pdf}}
    % \subfigure[Wide-ResNet-28-10 on CIFAR-100+]{
    %     \label{fig:evluationC100}
    % \includegraphics[width=0.45\columnwidth]{wrnc100.pdf}}
    \caption{Comparison with state-of-the-art image classification methods.}
    \label{compare}
    \end{center}
    \vskip -0.2in
\end{figure}

Curves of test errors of state-of-the-art methods and ISDA are presented in Figure \ref{compare}. ISDA outperforms other methods consistently, and shows the best generalization performance in all situations. Notably, ISDA decreases test errors more evidently in CIFAR-100, which demonstrates that our method is more suitable for datasets with fewer samples. This observation is consistent with the results in the paper. In addition, among other methods, center loss shows competitive performance with ISDA on CIFAR-10, but it fails to significantly enhance the generalization in CIFAR-100.
